# Supplementary material for: Dynamics of certain non-conformal degree two maps on the plane
Source: arXiv:math/9201293 source file (1991-09-26)
Supplement: Supplementary file 1 [file appendix.tex]

\ifx\macrosLoaded\undefined 
        \input ralfamac
\fi
\secno=-1 %% don't number this guy...
%**end of header
\section{Appendix}

We present here the numerical evidence which indicates the type of Hopf
bifurcation that occurs near the fixed point $z_0$ of $f_{\alpha,c}$
in the case where the derivative at $z_0$ has two complex conjugate
eigenvalues of norm 1. (See section 4).

One can change coordinates so that $f$ becomes
$$
F(z)= \mu z + b_2 z^2\bar z + O(|z|^5)
$$
where $|\mu|=1$ and $\mu$ is not a first, second, third, or fourth root of
unity. The type of Hopf bifurcation is given by the sign of the real part
of $b_2/\mu$.  In theory this is not hard to figure out, but in practice 
calculating the coordinate change is a horrendous task.  We use {\it
Mathematica} \cite{W} to do this.  The following is the {\it Mathematica}
session that we base our findings on.  The {\it Mathematica} session will be
printed in {\tt typewriter font} and comments will be made in the ordinary
roman font. 
\medskip

\noindent
We let $w=\bar z$ and 
${\tt Q2}(re^{i\theta})=r^{2\alpha}e^{2i\theta}=Q_\alpha^2$.            

\verbatim
Q2[{z_,w_},alpha_]:=z^(alpha + 1) w^(alpha - 1)
endverbatim

\noindent
The following procedure finds the terms of the Taylor expansion of $Q_\alpha^2$
up to degree 3 centered at $z_0$. Later $z_0$ will be a fixed point
of $f_{\alpha,c}(z)=Q_\alpha^2(z)+c$ with the appropriate kind of derivative.
The constant $c$ doesn't appear in what follows because $c$ will be determined
by $c=Q_\alpha^2(z_0)-z_0$, where $D_{z_0} Q_\alpha^2$ is of the right form.
\verbatim
Jet[z0_,alpha_]:=
    Expand[Normal[Series[
        Q2[{z+z0,w+Conjugate[z0]},alpha]-Q2[{z0,Conjugate[z0]},alpha],
        {z,0,3},{w,0,3}]]]
endverbatim

\noindent
We only want terms of total degree 3.  Chop off terms such as $z^2 w^3$.

\verbatim
ChopJet3[TheJet_] := 
    Block[{Jet = Expand[TheJet]}, 
         Return[Expand[Normal[Coefficient[Jet, w^3 ] + O[z]] w^3  + 
             Normal[Coefficient[Jet, w^2 ] + O[z]^2 ] w^2  + 
             Normal[Coefficient[Jet, w] + O[z]^3 ] w + 
             Normal[(Jet /. {w -> 0}) + O[z]^4 ]]]]
endverbatim

\noindent
The following function returns the conjugate of a jet.  For instance,
{\tt ConjJet}$(a + b\bar z^2 + c\bar z z^2) =
   \bar a + \bar b z^2 + \bar c z\bar z^2$. 
{\tt ExpJet[[i]][[1]]} is the coefficient of the ${\tt i}^{\rm th}$ term
in the jet and {\tt ExpJet[[i]]} is the ${\tt i}^{\rm th}$ term. 
For instance, {\tt ExpJet[[i]]} might be $c z^2 w$ ($w=\bar z$), then
{\tt ExpJet[[i]][[1]]} would be $c$.  Thus, we take each term in
the jet and conjugate each coefficient, and then switch $z$ with $w$. 

\verbatim
ConjJet[TheJet_] :=
  Block[{NJet=0,ExpJet=Expand[TheJet]},
    For[i=1, i<=Length[ExpJet], i++,
       NJet += Conjugate[ExpJet[[i]][[1]]] ExpJet[[i]]/ExpJet[[i]][[1]];
    ];
    NJet=NJet /. {w->z,z->w};
    Return[NJet]]
endverbatim

\noindent
The following changes coordinates so that a jet of the form 
$ a z + b \bar z + \ldots$  becomes $\lambda z + \ldots$  (no $\bar z^1$
term). The conjugation is $z= c \zeta + \bar \zeta$, where $\bar b c^2 +
(\bar a - a) c - b = 0$. This has an inverse if $|c|$ is not 1, which is the
case when $|b| < |\im a|$ or the derivative has complex conjugate 
eigenvalues. In practice (due to round off error) {\tt NewJet} will  have a
very small $\bar z$ term.  The function {\tt Chop} chops off such very small
terms.   

\verbatim
CoordChange1[MyJet_]:=
  Block[{a=Coefficient[MyJet,z]/.{w->0},
         b=Coefficient[MyJet,w]/.{z->0},
         c,temp,NewJet,},
     temp=a-Conjugate[a];
     c=(temp+Sqrt[temp^2+4 b Conjugate[b]])/(2 Conjugate[b]);
     NewJet=MyJet/. {z-> c z + w,w-> z + Conjugate[c] w};
     NewJet=(Conjugate[c] NewJet - ConjJet[NewJet])/(c Conjugate[c] -1);
     Return[Chop[ChopJet3[NewJet]]]]
endverbatim

\noindent
Compose the jets as functions.

\verbatim
ComposeJets[Jet1_,Jet2_]:=ChopJet3[Jet1 /. {z->Jet2,w->ConjJet[Jet2]}]
endverbatim

\noindent
The following procedure takes a jet and first changes coordinates  using
{\tt CoordChange1} so that the $w$ ($=\bar z)$ coefficient is 0. For
this we require the eigenvalues to be complex conjugate; if they are not this
routine produces nonsense. Secondly we change coordinates so that the
quadratic terms disappear.  For this we need that the eigenvalues  are not
first or third roots of unity.  If the eigenvalues are not second, third, or
fourth roots of unity we could also get rid of the $b_1$, $b_3$, and $b_4$
coordinates yielding the right normal form.  We don't actually need to do
these coordinate changes because they don't affect the $z^2 w$ coefficient.
We then return the $z^2 w$ coefficient divided by the $z$ coefficient.  The
sign of the real part determines the type of Hopf bifurcation. (If it is 0,
this is not a Hopf bifurcation). 

\verbatim
NormalForm3[TheJet_]:=
  Block[{a1,a2,a3, b1,b2,b3,b4, equ1,equ2,equ3,equ4, BigJet, aRule,
        L1, returnJet, u, NormalJet},
     returnJet=ChopJet3[TheJet];
     returnJet=CoordChange1[returnJet];
     u=Coefficient[returnJet,z] /. {w->0};
     L1=2z + a1 z^2 + a2 z w + a3 w^2;
     NormalJet=u z + b1 z^3 + b2 z^2 w + b3 z w^2 + b4 w^3;
     BigJet= ComposeJets[returnJet,L1]-ComposeJets[L1,NormalJet];
     equ1= ((Coefficient[BigJet,z^2] /. {w->0}) ==0);
     equ2= (Coefficient[BigJet,z w]==0);
     equ3= ((Coefficient[BigJet,w^2] /. {z->0}) ==0);
     aRule=Solve[{equ1,equ2,equ3},{a1,a2,a3}];
     a1=a1/. aRule;
     a2=a2/. aRule;
     a3=a3/. aRule;
     equ4= (Coefficient[BigJet,z^2 w]  ==0);
     b2=b2 /. Solve[equ4,b2])[[1]];
     Return[b2/u]]
endverbatim

\noindent
The determinant of $D_z Q_\alpha^2$ is $4\alpha (z w)^{2\alpha - 1}$, and
the trace of $D_zQ_\alpha^2$ is	$(\alpha + 1)(z w)^{\alpha - 1}(z + w)$.
We want to find $z$ so that  $D_z Q_\alpha^2$ has eigenvalues 
$\e^{\pm\i\theta}$; that is, the determinant is 1 and the trace is
$2\cos\theta$, so 
$$|z|=(4\alpha)^{{1}\over{2-4\alpha}}
      \hbox{\quad and \quad}
  \arg(z)=\cos^{-1}\( 
    {(4\alpha)^{{\alpha-1}\over{2\alpha-1}}
      \over{\alpha + 1}} \cos\theta\).
$$
Then return the real part of {\tt NormalForm3[Jet[$z,\alpha$]]]},
which we will call the Hopf number. 

\verbatim
DoNormalForm3[theta_, alpha_] :=
   Block[{zee,r,argz},
     r=(4alpha)^(1/(2-4alpha));
     argz=Cos[theta](4alpha)^((alpha-1)/(2alpha-1))/(alpha + 1);
     If[Abs[argz]>1,
        Print["Eigenvalues of ",theta," are not complex conjugates."];
        Return[0]];
     argz=ArcCos[argz];
     zee=r E^(I argz);
     Return[Re[NormalForm3[Jet[zee,alpha]]]]]
endverbatim

\noindent
We now make a plot of the Hopf numbers as a function of $\theta$ and $\beta$,
where $\alpha=1/(1-\beta)$ is a coordinate change sending
$\alpha=1/2,1,\infty$ to $\beta=-1,0,1$ respectively. This coordinate change
allows us to better see the behavior for the full range of values of $\alpha$.
We deal with $\beta < 0$ and $\beta>0$ separately, because of the
discontinuity at the conformal case ($\beta=0$ or $\alpha=1$).
\verbatim
neg  =Plot3D[DoNormalForm3[theta,1/(1-beta)], {beta,-.995,-.005},
           {theta,0,2 Pi}, DisplayFunction->Identity];
pos  =Plot3D[DoNormalForm3[theta,1/(1-beta)], {beta,.005,.995}, 
           {theta,0,2 Pi}, DisplayFunction->Identity];
endverbatim

\noindent
Finally we display the picture.  Notice that for $\beta<0$ or $\alpha<1$ the
Hopf numbers are positive, and for $\beta>0$ or $\alpha>1$ the Hopf numbers
are negative.  To emphasize this, we display a blowup near 0, and include
the plane dividing the positive values from the negative ones.

\midinsert{
  \centerline{\psfig{figure=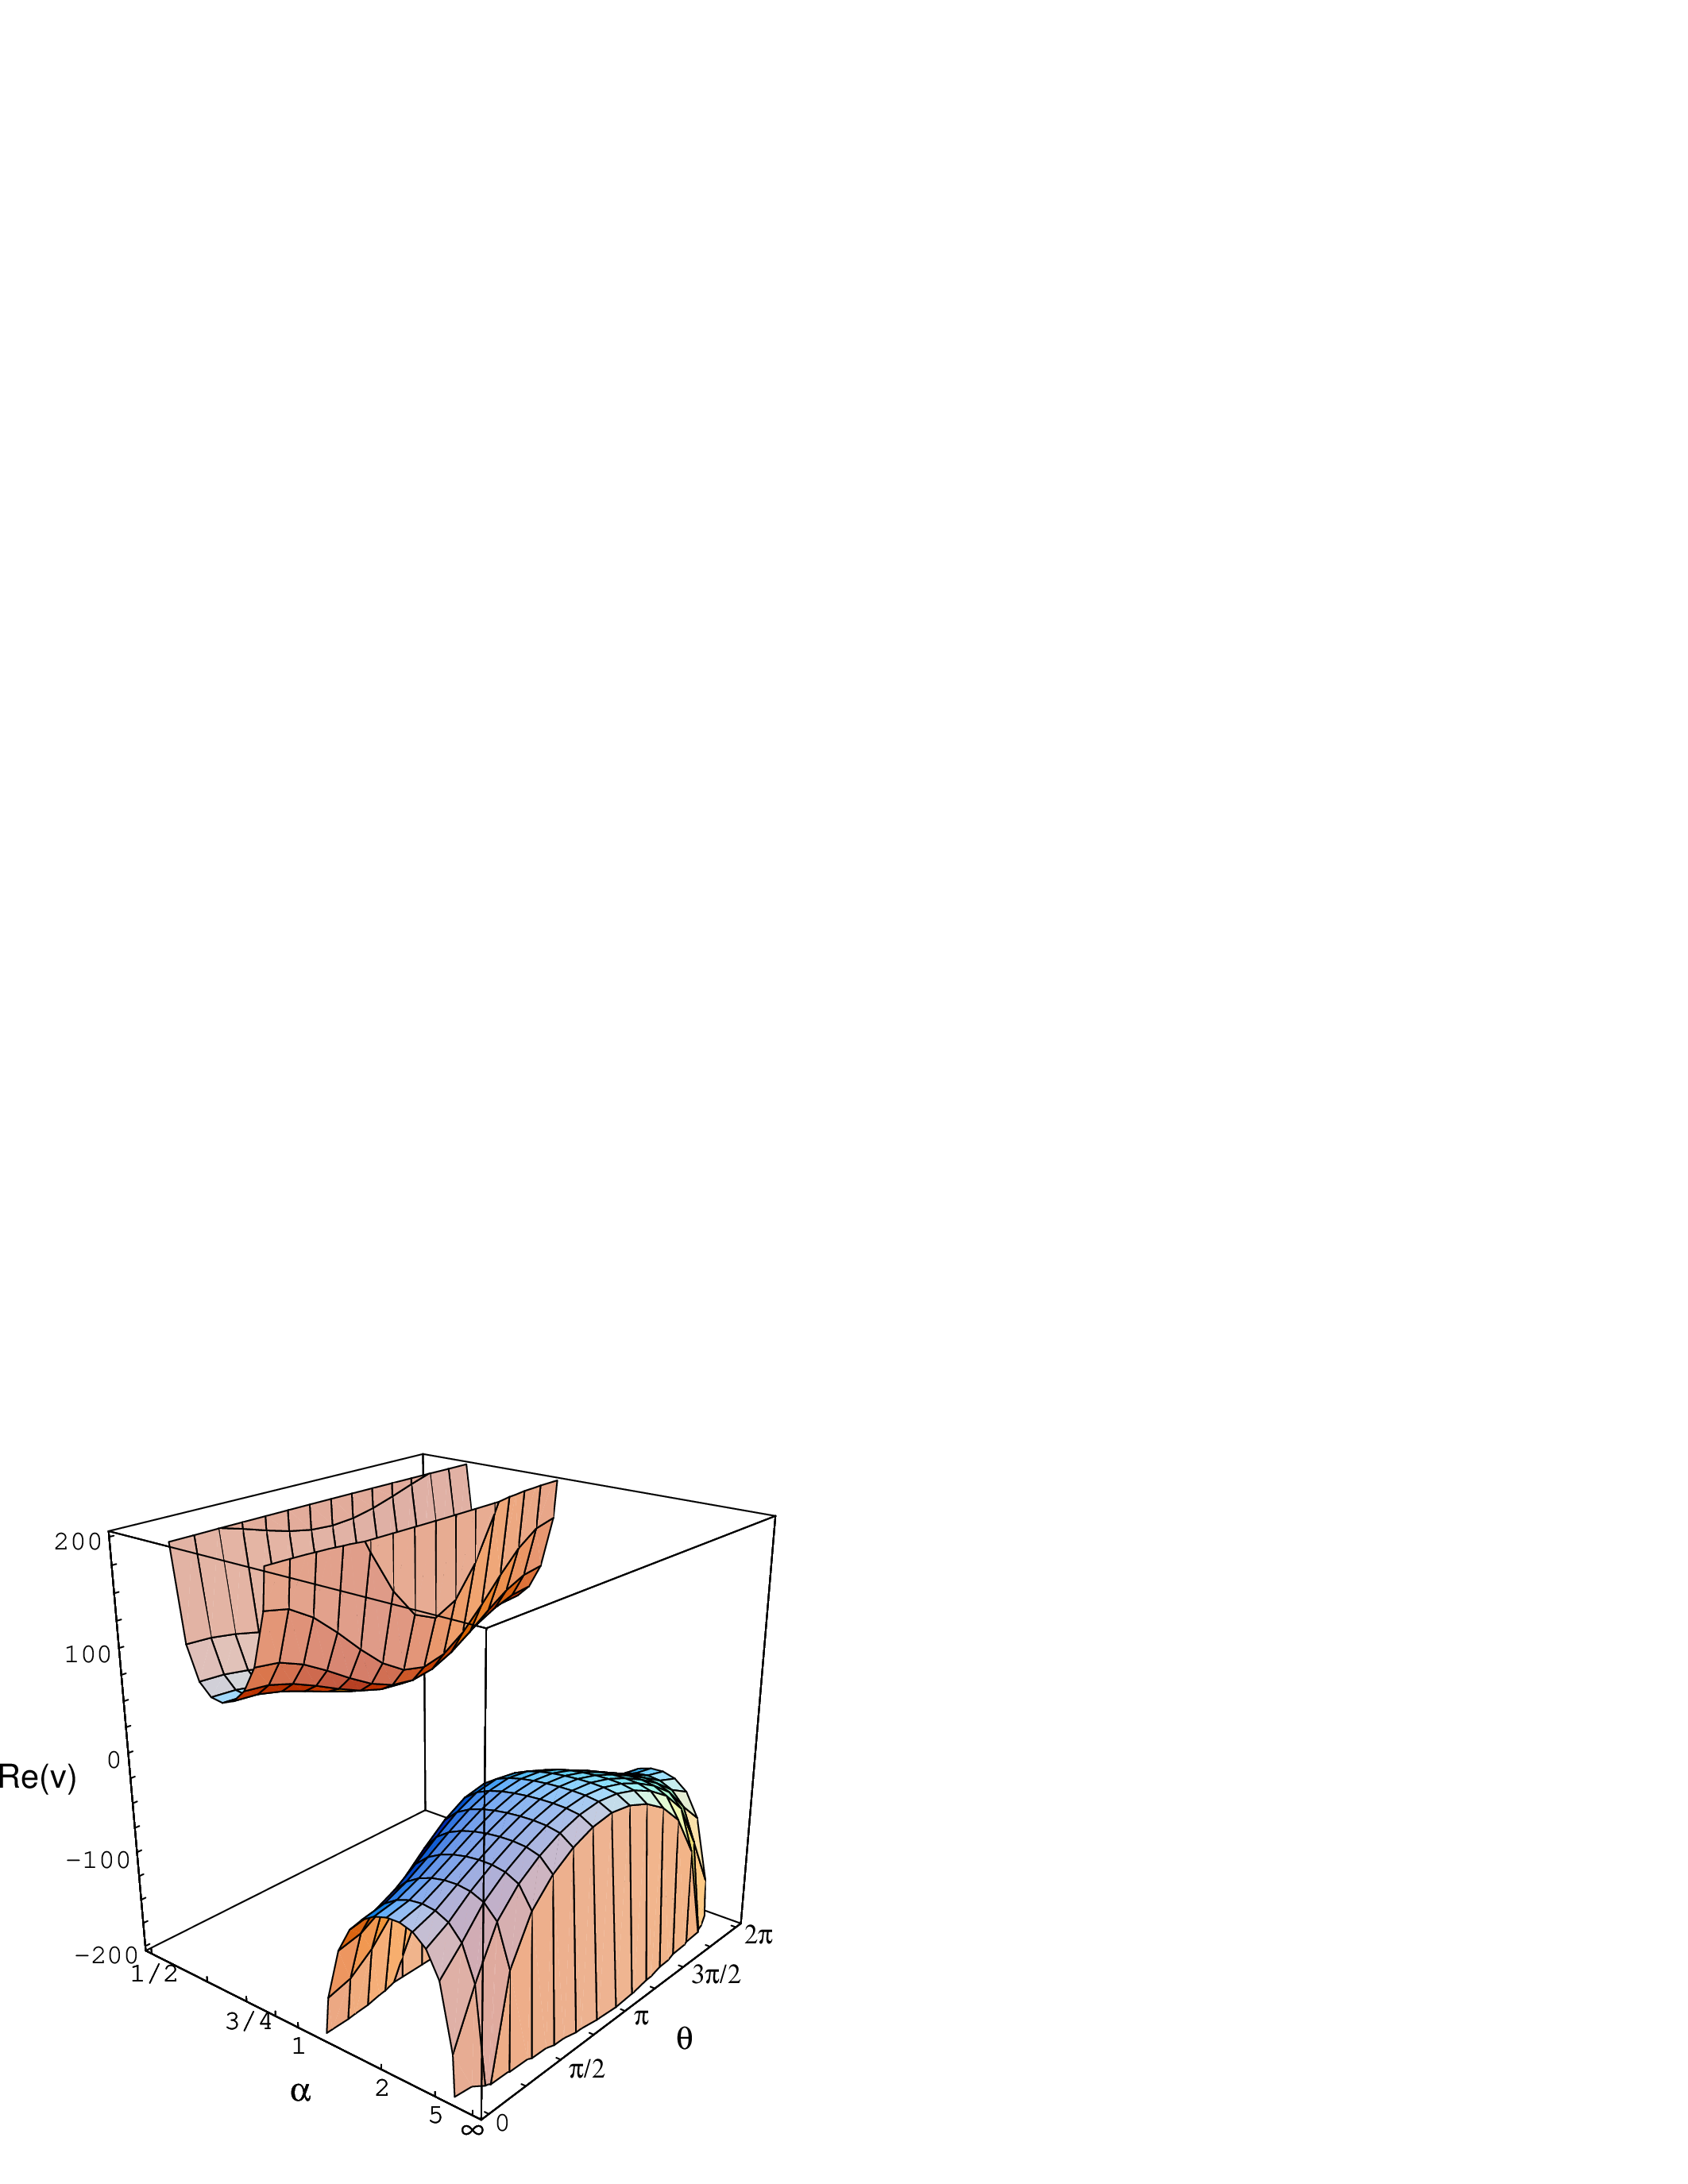,height=.48\hsize}\hfil
	      \psfig{figure=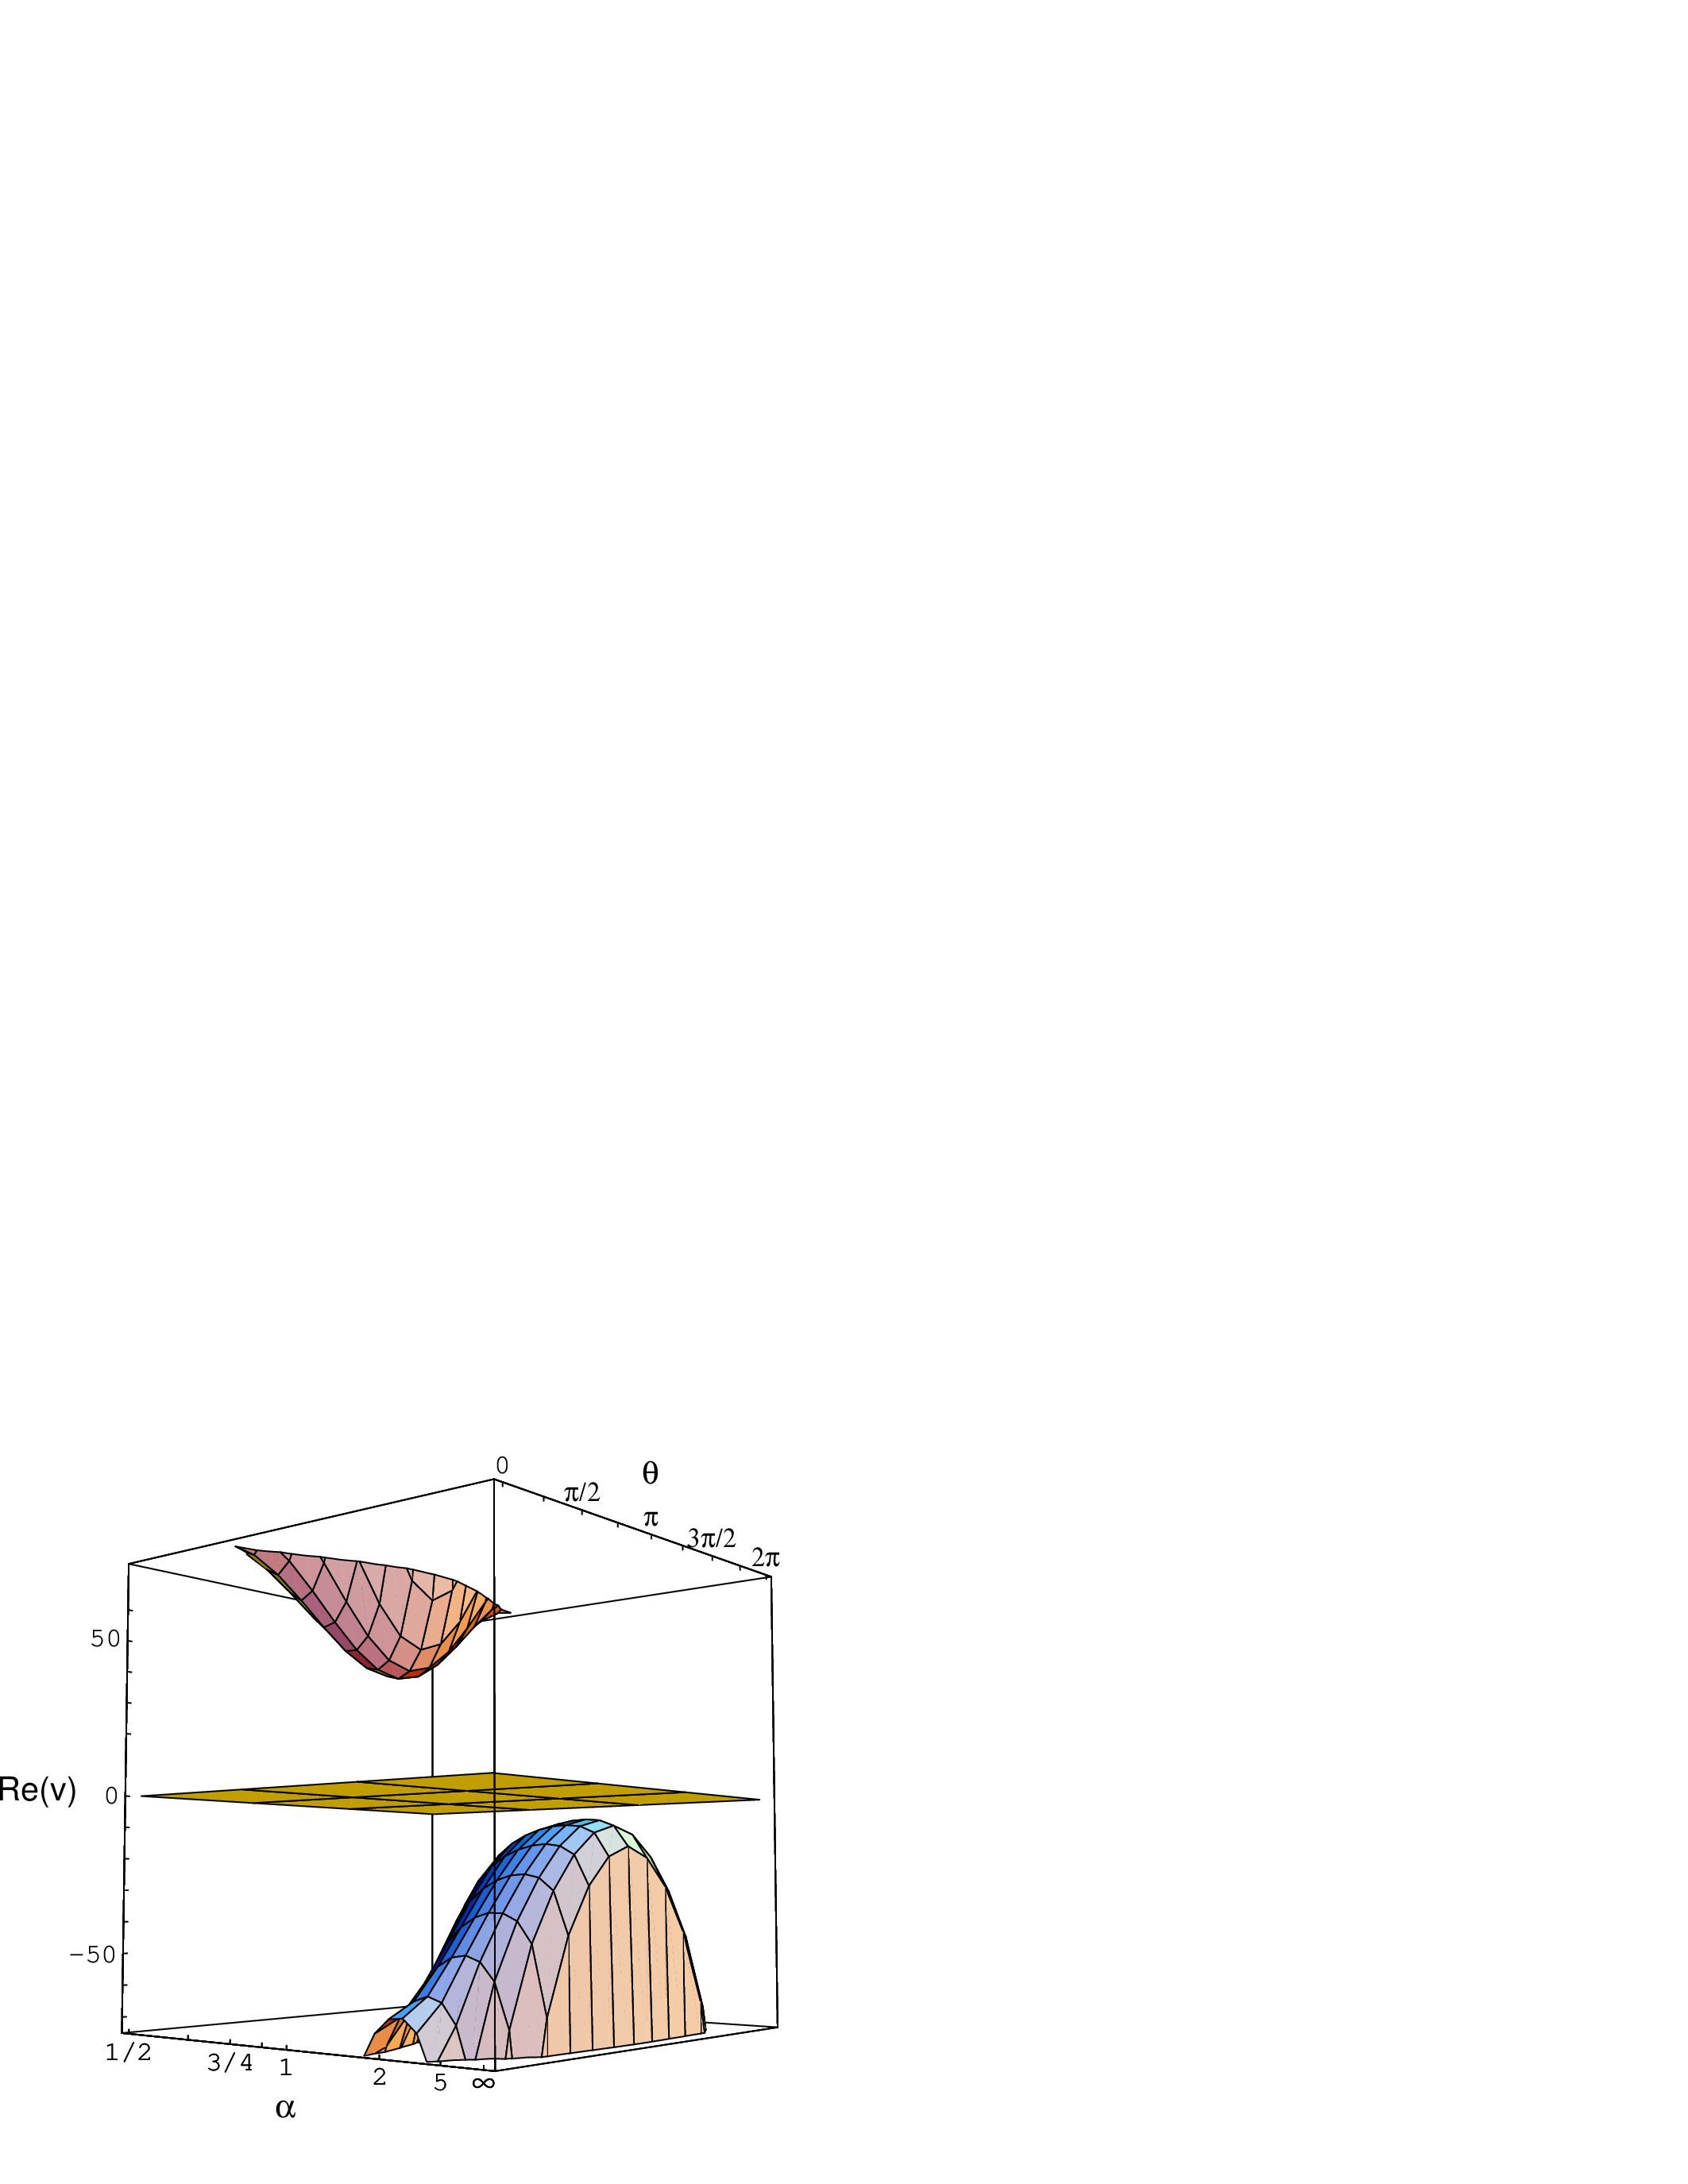,height=.48\hsize}}
   \shortcaption{The graph of the Hopf numbers, and a blowup near the
   $Hopf=0$ plane.} 
}\endinsert

\verbatim
Show[{neg,pos}, DisplayFunction->$DisplayFunction,
        ViewPoint->{2.0,-2.4,1.3}, 
        BoxRatios->{1,1,1}, PlotRange->{-205,205},
        AxesLabel->{FontForm["b",{"Symbol",10}],
                    FontForm["q",{"Symbol",10}],
                    "Hopf"}];
plane=Plot3D[0,{beta,-1,1}, {theta,0,2 Pi},PlotPoints->4,
         DisplayFunction->Identity];
Show[{neg,pos,plane},DisplayFunction->$DisplayFunction,
        ViewPoint->{2.0,-2.4,-0.2}, 
        BoxRatios->{1,1,1}, PlotRange->{-75,75},
        AxesLabel->{FontForm["b",{"Symbol",10}],
                    FontForm["q",{"Symbol",10}],
                    "Hopf"}];
endverbatim
